# Supplementary material for: Rank-one Convexification for Sparse Regression
Source: arXiv:1901.10334 source file (2020-10-18)
Supplement: Supplementary file 1 [file appendix.tex]

\clearpage
\appendix
\section{Detailed computational results on real instances}\label{sec:appendix}
\begin{table}
	\caption{Best subset selection on \texttt{housing} instances, $n=506$, $p=13$, $E_d=26.7\%$, $E_{sdd}=48.6\%$.}
	\begin{tabular}{c c c l| c c c c c c c c}
		\hline
		\multirow{2}{*}{$\lambda$ } & \multirow{2}{*}{$k$ }& \multirow{2}{*}{\texttt{method}}&\multirow{2}{*}{$|T|$}&\multicolumn{3}{c}{\underline{\texttt{objective}}}& \multirow{2}{*}{\texttt{nonzero}}& \multirow{2}{*}{\texttt{time}}\\
		&&&&\texttt{LB}&\texttt{UB}&\texttt{gap}\\
		\hline   
		\multirow{11}{*}{\texttt{$0.00$}}&\multirow{11}{*}{$3$}&\texttt{ols}&0 & 80.7 & 154.4 & 91.3& 13 & 0.0\\
		&&&&&&&&&&\\
		&&\multirow{4}{*}{\texttt{socp}}&1 & 98.7 & 100.5 & 1.8& 12 & 0.1\\
		&&&2-& 99.8 & 100.1 & 0.3&13 & 0.1 \\
		&&&2 & 100.0 & 100.0 & 0.0&12 & 0.1\\
		&&&3& 100.0 & 100.0 & 0.0&3 & 0.3 \\
		&&&&&&&&&&\\
		&&\multirow{4}{*}{\texttt{sdp}}&1 & 99.8 & 100.1 & 0.2& 8 & 0.0\\
		&&&2 & 100.0 & 100.0 & 0.0&3 & 0.0\\
		&&&2 & 100.0 & 100.0 & 0.0&3 & 0.0\\
		&&&3 & 100.0 & 100.0 & 0.0&3 & 0.2\\
		\hline
		\multirow{11}{*}{\texttt{$0.00$}}&\multirow{11}{*}{$5$}&\texttt{ols}&0& 88.8 & 179.7 & 102.2 & 13 & 0.0\\
		&&&&&&&&&&\\
		&&\multirow{4}{*}{\texttt{socp}}&1& 98.6 & 100.5 & 2.0 & 13 & 0.1\\
		&&&2-&99.5 & 100.6 & 1.1 & 12 & 0.1\\
		&&&2&99.7 & 100.5 & 0.8 & 13 & 0.8\\
		&&&3&100.0 & 100.1 & 0.1 & 12 & 0.3\\
		&&&&&&&&&&\\
		&&\multirow{4}{*}{\texttt{sdp}}&1& 100.0 & 100.0 & 0.0 & 5 & 0.0\\
		&&&2-&100.0 & 100.0 & 0.0 & 5 & 0.0\\
		&&&2&100.0 & 100.0 & 0.0 & 5 & 0.0\\
		&&&3&100.0 & 100.0 & 0.0 & 5 & 0.2\\
		\hline
		\multirow{11}{*}{\texttt{$0.05$}}&\multirow{11}{*}{$5$}&\texttt{ridge}&0& 90.9 & 156.1 & 71.8 & 13 & 0.0\\
		&&&&&&&&&&\\
		&&\multirow{4}{*}{\texttt{socp}}&1& 98.9 & 100.8 & 2.0 & 11 & 0.1\\
		&&&2-&99.7 & 100.9 & 1.2 & 12 & 0.1\\
		&&&2&99.8 & 100.9 & 1.1 & 13 & 0.1\\
		&&&3&100.0 & 100.3 & 0.4 & 13 & 0.3\\
		&&&&&&&&&&\\
		&&\multirow{4}{*}{\texttt{sdp}}&1& 99.9 & 100.3 & 0.4 & 10 & 5\\
		&&&2-&100.0 & 100.0 & 0.0 & 5 & 0.0\\
		&&&2&100.0 & 100.0 & 0.0 & 5 & 0.0\\
		&&&3&100.0 & 100.0 & 0.0 & 6 & 0.2\\
		\hline
	\end{tabular}
\end{table}

\begin{table}
	\caption{Best subset selection on \texttt{servo} instances, $n=167$, $p=19$, $E_d=0.0\%$, $E_{sdd}=62.0\%$.}
	\begin{tabular}{c c c l| c c c c c c c c}
		\hline
		\multirow{2}{*}{$\lambda$ } & \multirow{2}{*}{$k$ }& \multirow{2}{*}{\texttt{method}}&\multirow{2}{*}{$|T|$}&\multicolumn{3}{c}{\underline{\texttt{objective}}}& \multirow{2}{*}{\texttt{nonzero}}& \multirow{2}{*}{\texttt{time}}\\
		&&&&\texttt{LB}&\texttt{UB}&\texttt{gap}\\
		\hline   
		\multirow{11}{*}{\texttt{$0.00$}}&\multirow{11}{*}{$3$}&\texttt{ols}&0& 77.4 & 173.2 & 123.6 & 0.0 & 19\\
		&&&&&&&&&&\\
		&&\multirow{4}{*}{\texttt{socp}}&1& 77.4 & 133.2 & 72.1 & 19 & 0.0\\
		&&&2-&77.4 & 164.5 & 112.5 & 19 & 0.1\\
		&&&2&77.4 & 133.4 & 72.3 & 19 & 0.1\\
		&&&3&77.4 & 135.6 & 75.1 & 19 & 0.6\\
		&&&&&&&&&&\\
		&&\multirow{4}{*}{\texttt{sdp}}&1& 77.4 & 162.1 & 109.4 & 19 & 0.0\\
		&&&2-&77.4 & 626.7 & 709.2 & 19 & 0.1\\
		&&&2&99.7 & 100.0 & 0.3 & 14 & 0.1\\
		&&&3&99.8 & 100.0 & 0.3 & 15 & 1.0\\
		\hline
		\multirow{11}{*}{\texttt{$0.00$}}&\multirow{11}{*}{$5$}&\texttt{ols}&0& 84.1 & 141.5 & 68.4 & 19 & 0.0\\
		&&&&&&&&&&\\
		&&\multirow{4}{*}{\texttt{socp}}&1& 84.1 & 131.0 & 55.8 & 19 & 0.0\\
		&&&2-&84.1 & 139.2 & 65.6 & 19 & 0.1\\
		&&&2&84.1 & 134.2 & 59.6 & 19 & 0.1\\
		&&&3&84.1 & 136.0 & 61.8 & 19 & 0.5\\
		&&&&&&&&&&\\
		&&\multirow{4}{*}{\texttt{sdp}}&1& 84.1 & 130.9 & 55.7 & 19 & 0.0\\
		&&&2-&84.1 & 479.4 & 470.4 & 19 & 0.1\\
		&&&2&96.1 & 100.3 & 4.4 & 15 & 0.1\\
		&&&3&96.2 & 100.0 & 4.0 & 14 & 0.8\\
		\hline
		\multirow{11}{*}{\texttt{$0.05$}}&\multirow{11}{*}{$5$}&\texttt{ridge}&0& 87.2 & 122.9 & 40.9 & 19 & 0.0\\
		&&&&&&&&&&\\
		&&\multirow{4}{*}{\texttt{socp}}&1& 92.4 & 103.9 & 12.4 & 14 & 0.0\\
		&&&2-&93.5 & 104.1 & 11.4 & 19 & 0.1\\
		&&&2&93.8 & 103.9 & 10.7 & 19 & 0.1\\
		&&&3&96.5 & 103.7 & 7.4 & 19 & 0.8\\
		&&&&&&&&&&\\
		&&\multirow{4}{*}{\texttt{sdp}}&1& 93.3 & 103.0 & 10.4 & 19 & 0.0\\
		&&&2-&99.4 & 100.0 & 0.6 & 15 & 0.1\\
		&&&2&99.5 & 100.0 & 0.5 & 16 & 0.1\\
		&&&3&99.6 & 100.0 & 0.4 & 11 & 0.9\\
		\hline
	\end{tabular}
\end{table}

\begin{table}
	\caption{Best subset selection on \texttt{autoMPG} instances, $n=392$, $p=25$, $E_d=1.5\%$, $E_{sdd}=59.9\%$.}
	\begin{tabular}{c c c l| c c c c c c c c}
		\hline
		\multirow{2}{*}{$\lambda$ } & \multirow{2}{*}{$k$ }& \multirow{2}{*}{\texttt{method}}&\multirow{2}{*}{$|T|$}&\multicolumn{3}{c}{\underline{\texttt{objective}}}& \multirow{2}{*}{\texttt{nonzero}}& \multirow{2}{*}{\texttt{time}}\\
		&&&&\texttt{LB}&\texttt{UB}&\texttt{gap}\\
		\hline   
		\multirow{11}{*}{\texttt{$0.00$}}&\multirow{11}{*}{$3$}&\texttt{ols}&0& 56.6 & 114.0 & 101.4 & 25 & 0.0\\
		&&&&&&&&&&\\
		&&\multirow{4}{*}{\texttt{socp}}&1& 56.6 & 117.1 & 106.9 & 23 & 0.3\\
		&&&2-&56.6 & 116.6 & 105.9 & 24 & 0.4\\
		&&&2&56.6 & 117.0 & 106.7 & 24 & 0.5\\
		&&&3&57.1 & 120.3 & 110.9 & 25 & 3.2\\
		&&&&&&&&&&\\
		&&\multirow{4}{*}{\texttt{sdp}}&1& 56.6 & 114.3 & 101.9 & 24 & 0.1\\
		&&&2-&79.3 & 181.8 & 129.2 & 24 & 0.2\\
		&&&2&99.3 & 100.4 & 1.1 & 16 & 0.2\\
		&&&3&99.6 & 100.0 & 0.4 & 9 & 2.8\\
		\hline
		\multirow{11}{*}{\texttt{$0.00$}}&\multirow{11}{*}{$5$}&\texttt{ols}&0& 71.4 & 142.7 & 99.8 & 25 & 0.0\\
		&&&&&&&&&&\\
		&&\multirow{4}{*}{\texttt{socp}}&1& 71.4 & 142.6 & 99.8 & 25 & 0.2\\
		&&&2-&71.4 & 141.5 & 98.3 & 25 & 0.9\\
		&&&2&71.4 & 141.5 & 98.2 & 25 & 0.3\\
		&&&3&71.4 & 140.5 & 96.8 & 25 & 3.3\\
		&&&&&&&&&&\\
		&&\multirow{4}{*}{\texttt{sdp}}&1& 71.4 & 144.6 & 102.5 & 25 & 0.0\\
		&&&2-&78.5 & 384.1 & 389.6 & 25 & 0.3\\
		&&&2&99.4 & 101.8 & 2.4 & 22 & 0.2\\
		&&&3&100.0 & 100.0 & 0.0 & 6 & 2.7\\
		\hline
		\multirow{11}{*}{\texttt{$0.05$}}&\multirow{11}{*}{$5$}&\texttt{ridge}&0& 70.8 & 125.7 & 77.7 & 25 & 0.0\\
		&&&&&&&&&&\\
		&&\multirow{4}{*}{\texttt{socp}}&1& 80.4 & 109.0 & 35.6 & 17 & 0.2\\
		&&&2-&88.8 & 113.0 & 27.3 & 24 & 1.0\\
		&&&2&90.4 & 110.8 & 22.5 & 25 & 0.3\\
		&&&3&94.4 & 108.5 & 14.9 & 25 & 2.0\\
		&&&&&&&&&&\\
		&&\multirow{4}{*}{\texttt{sdp}}&1& 84.0 & 115.5 & 37.6 & 25 & 0.0\\
		&&&2-&99.1 & 105.4 & 6.4 & 20 & 0.2\\
		&&&2&99.7 & 101.2 & 1.5 & 19 & 0.2\\
		&&&3&99.9 & 100.0 & 0.1 & 7 & 2.8\\
		\hline
	\end{tabular}
\end{table}

\begin{table}
	\caption{Best subset selection on \texttt{solar flare} instances, $n=1,066$, $p=26$, $E_d=8.8\%$, $E_{sdd}=47.0\%$.}
	\begin{tabular}{c c c l| c c c c c c c c}
		\hline
		\multirow{2}{*}{$\lambda$ } & \multirow{2}{*}{$k$ }& \multirow{2}{*}{\texttt{method}}&\multirow{2}{*}{$|T|$}&\multicolumn{3}{c}{\underline{\texttt{objective}}}& \multirow{2}{*}{\texttt{nonzero}}& \multirow{2}{*}{\texttt{time}}\\
		&&&&\texttt{LB}&\texttt{UB}&\texttt{gap}\\
		\hline   
		\multirow{11}{*}{\texttt{$0.00$}}&\multirow{11}{*}{$3$}&\texttt{ols}&0& 94.7 & 102.5 & 8.3 & 26 & 0.0\\
		&&&&&&&&&&\\
		&&\multirow{4}{*}{\texttt{socp}}&1& 94.7 & 102.6 & 8.4 & 26 & 0.7\\
		&&&2-&94.7 & 102.4 & 8.2 & 26 & 0.8\\
		&&&2&94.7 & 100.6 & 6.2 & 26 & 0.5\\
		&&&3&94.7 & 102.4 & 8.2 & 26 & 2.0\\
		&&&&&&&&&&\\
		&&\multirow{4}{*}{\texttt{sdp}}&1& 94.7 & 103.8 & 9.7 & 25 & 0.1\\
		&&&2-&94.8 & 117.7 & 24.1 & 26 & 0.3\\
		&&&2&97.6 & 100.4 & 2.9 & 20 & 0.3\\
		&&&3&97.8 & 100.0 & 2.3 & 19 & 3.1\\
		\hline
		\multirow{11}{*}{\texttt{$0.00$}}&\multirow{11}{*}{$5$}&\texttt{ols}&0& 97.5 & 103.9 & 6.6 & 26 & 0.0\\
		&&&&&&&&&&\\
		&&\multirow{4}{*}{\texttt{socp}}&1& 97.5 & 104.3 & 6.9 & 26 & 0.7\\
		&&&2-&97.5 & 103.7 & 6.3 & 26 & 0.5\\
		&&&2&97.5 & 103.3 & 5.9 & 26 & 0.8\\
		&&&3&97.5 & 103.9 & 6.6 & 25 & 1.9\\
		&&&&&&&&&&\\
		&&\multirow{4}{*}{\texttt{sdp}}&1& 97.5 & 107.8 & 10.5 & 26 & 0.0\\
		&&&2-&97.5 & 117.2 & 20.2 & 26 & 0.3\\
		&&&2&98.9 & 100.0 & 1.1 & 20 & 0.3\\
		&&&3&98.9 & 100.0 & 1.1 & 19 & 2.8\\
		\hline
		\multirow{11}{*}{\texttt{$0.05$}}&\multirow{11}{*}{$5$}&\texttt{ridge}&0& 97.8 & 102.5 & 4.8 & 26 & 0.0\\
		&&&&&&&&&&\\
		&&\multirow{4}{*}{\texttt{socp}}&1& 98.5 & 100.5 & 2.0 & 16 & 0.7\\
		&&&2-&98.8 & 100.5 & 1.7 & 25 & 0.6\\
		&&&2&98.9 & 100.5 & 1.6 & 25 & 0.9\\
		&&&3&99.3 & 100.5 & 1.1 & 24 & 2.6\\
		&&&&&&&&&&\\
		&&\multirow{4}{*}{\texttt{sdp}}&1& 99.0 & 100.4 & 1.4 & 24 & 0.0\\
		&&&2-&99.6 & 100.0 & 0.4 & 18 & 0.2\\
		&&&2&99.7 & 100.0 & 0.3 & 17 & 0.2\\
		&&&3&99.8 & 100.0 & 0.2 & 18 & 2.5\\
		\hline
	\end{tabular}
\end{table}

\begin{table}
	\caption{Best subset selection on \texttt{breast cancer} instances, $n=196$, $p=37$, $E_d=3.6\%$, $E_{sdd}=52.8\%$.}
	\begin{tabular}{c c c l| c c c c c c c c}
		\hline
		\multirow{2}{*}{$\lambda$ } & \multirow{2}{*}{$k$ }& \multirow{2}{*}{\texttt{method}}&\multirow{2}{*}{$|T|$}&\multicolumn{3}{c}{\underline{\texttt{objective}}}& \multirow{2}{*}{\texttt{nonzero}}& \multirow{2}{*}{\texttt{time}}\\
		&&&&\texttt{LB}&\texttt{UB}&\texttt{gap}\\
		\hline   
		\multirow{11}{*}{\texttt{$0.00$}}&\multirow{11}{*}{$3$}&\texttt{ols}&0& 83.8 & 102.4 & 22.2 & 36 & 0.0\\
		&&&&&&&&&&\\
		&&\multirow{4}{*}{\texttt{socp}}&1& 83.8 & 102.4 & 22.2 & 36 & 0.1\\
		&&&2-&83.8 & 102.5 & 22.3 & 36 & 0.3\\
		&&&2&83.8 & 102.4 & 22.2 & 36 & 0.4\\
		&&&3&83.8 & 105.9 & 26.4 & 36 & 7.2\\
		&&&&&&&&&&\\
		&&\multirow{4}{*}{\texttt{sdp}}&1& 83.8 & 106.1 & 26.6 & 36 & 0.1\\
		&&&2-&84.3 & 258.8 & 207.1 & 36 & 0.6\\
		&&&2&98.6 & 100.6 & 2.0 & 33 & 0.6\\
		&&&3&99.1 & 100.0 & 0.9 & 30 & 8.4\\
		\hline
		\multirow{11}{*}{\texttt{$0.00$}}&\multirow{11}{*}{$5$}&\texttt{ols}&0& 86.2 & 101.4 & 17.7 & 36 & 0.0\\
		&&&&&&&&&&\\
		&&\multirow{4}{*}{\texttt{socp}}&1& 86.2 & 101.5 & 17.8 & 36 & 0.1\\
		&&&2-&86.2 & 101.5 & 17.8 & 36 & 0.4\\
		&&&2&86.2 & 101.4 & 17.7 & 36 & 0.4\\
		&&&3&86.2 & 101.5 & 17.8 & 36 & 6.7\\
		&&&&&&&&&&\\
		&&\multirow{4}{*}{\texttt{sdp}}&1& 86.2 & 101.7 & 18.0 & 36 & 0.1\\
		&&&2-&86.3 & 275.5 & 219.2 & 36 & 0.7\\
		&&&2&97.2 & 100.5 & 3.5 & 34 & 0.7\\
		&&&3&97.6 & 100.0 & 2.5 & 31 & 8.3\\
		\hline
		\multirow{11}{*}{\texttt{$0.05$}}&\multirow{11}{*}{$5$}&\texttt{ridge}&0&87.9& 103.2 & 17.5 & 36 & 0.0 \\
		&&&&&&&&&&\\
		&&\multirow{4}{*}{\texttt{socp}}&1& 91.0 & 102.6 & 12.7 & 25 & 0.1\\
		&&&2-&92.6 & 102.7 & 11.0 & 35 & 0.4\\
		&&&2&92.8 & 102.8 & 10.8 & 36 & 0.5\\
		&&&3&95.4 & 102.9 & 7.9 & 36 & 7.8\\
		&&&&&&&&&&\\
		&&\multirow{4}{*}{\texttt{sdp}}&1& 93.1 & 102.8 & 10.4 & 35 & 0.1\\
		&&&2-&99.2 & 101.6 & 2.4 & 36 & 0.5\\
		&&&2&99.7 & 101.0 & 1.4 & 35 & 0.6\\
		&&&3&100.0 & 100.0 & 0.0 & 24 & 9.7\\
		\hline
	\end{tabular}
\end{table}

\begin{table}
	\caption{Best subset selection on \texttt{diabetes} instances, $n=442$, $p=64$, $E_d=0.0\%$, $E_{sdd}=17.7\%$.}
	\begin{tabular}{c c c l| c c c c c c c c}
		\hline
		\multirow{2}{*}{$\lambda$ } & \multirow{2}{*}{$k$ }& \multirow{2}{*}{\texttt{method}}&\multirow{2}{*}{$|T|$}&\multicolumn{3}{c}{\underline{\texttt{objective}}}& \multirow{2}{*}{\texttt{nonzero}}& \multirow{2}{*}{\texttt{time}}\\
		&&&&\texttt{LB}&\texttt{UB}&\texttt{gap}\\
		\hline   
		\multirow{11}{*}{\texttt{$0.00$}}&\multirow{11}{*}{$3$}&\texttt{ols}&0& 62.0 & 1,052.2 & 1,598.2 & 64 & 0.0\\
		&&&&&&&&&&\\
		&&\multirow{4}{*}{\texttt{socp}}&1& 62.0 & 1,052.5 & 1598.6 & 64 & 0.6\\
		&&&2-&62.0 & 2,168.0 & 3,398.8 & 64 & 2.7\\
		&&&2&62.0 & 2,115.9 & 3,314.8 & 64 & 4.1\\
		&&&3&62.1 & 490.8 & 690.1 & 64 & 100.1\\
		&&&&&&&&&&\\
		&&\multirow{4}{*}{\texttt{sdp}}&1& 69.9 & 189.2 & 170.6 & 62 & 3.3\\
		&&&2-&71.5 & 148.5 & 107.6 & 61 & 7.5\\
		&&&2&76.0 & 100.0 & 31.5 & 61 & 9.5\\
		&&&3&78.2 & 101.2 & 29.4 & 62 & 120.3\\
		\hline
		\multirow{11}{*}{\texttt{$0.00$}}&\multirow{11}{*}{$5$}&\texttt{ols}&0& 74.6 & 3,433.4 & 4,501.9 & 64 & 0.0\\
		&&&&&&&&&&\\
		&&\multirow{4}{*}{\texttt{socp}}&1& 74.6 & 3,433.6 & 4,502.1 & 64 & 0.5\\
		&&&2-&74.6 & 1,117.2 & 1,397.4 & 64 & 2.5\\
		&&&2&74.6 & 1,079.7 & 1,347.1 & 64 & 3.9\\
		&&&3&74.7 & 516.8 & 591.5 & 64 & 98.4\\
		&&&&&&&&&&\\
		&&\multirow{4}{*}{\texttt{sdp}}&1& 79.9 & 298.1 & 273.2 & 60 & 3.1\\
		&&&2-&81.2 & 121.6 & 49.7 & 59 & 8.2\\
		&&&2&85.2 & 100.9 & 18.5 & 61 & 9.0\\
		&&&3&87.7 & 100.0 & 14.0 & 60 & 125.5\\
		\hline
		\multirow{11}{*}{\texttt{$0.05$}}&\multirow{11}{*}{$5$}&\texttt{ridge}&0& 87.0 & 109.8 & 26.3 & 64 & 0.0\\
		&&&&&&&&&&\\
		&&\multirow{4}{*}{\texttt{socp}}&1& 93.1 & 100.0 & 7.4 & 32 & 0.6\\
		&&&2-&94.3 & 100.1 & 6.2 & 54 & 2.7\\
		&&&2&94.5 & 100.1 & 6.0 & 60 & 3.0\\
		&&&3&96.2 & 100.3 & 4.3 & 64 & 87.7\\
		&&&&&&&&&&\\
		&&\multirow{4}{*}{\texttt{sdp}}&1& 97.5 & 100.6 & 3.2 & 46 & 1.7\\
		&&&2-&99.0 & 100.8 & 1.7 & 48 & 5.3\\
		&&&2&99.2 & 100.7 & 1.6 & 47 & 4.8\\
		&&&3&99.6 & 100.6 & 1.0 & 41 & 101.0\\
		\hline
	\end{tabular}
\end{table}
